# Supplementary material for: Learning-Based Dimensionality Reduction for Computing Compact and Effective Local Feature Descriptors
Source: arXiv:2209.13586 source file (2022-09-27)
Supplement: Supplementary file 1 [file sift_aachen.tex]

\begin{figure}[htb!]
\centering
\def\iwidth{.49\linewidth}

\begin{minipage}{\iwidth}
    \centering
    \small{SIFT-PCA-64}
\end{minipage}%
\begin{minipage}{\iwidth}
    \centering
    \small{SIFT-Triplet-64}
\end{minipage}

\begin{minipage}{\iwidth}
    \centering
    \includegraphics[width=0.98\linewidth]{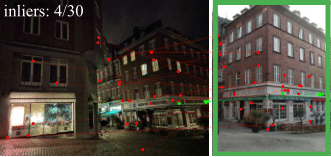}
\end{minipage}%
\begin{minipage}{\iwidth}
    \centering
    \includegraphics[width=0.98\linewidth]{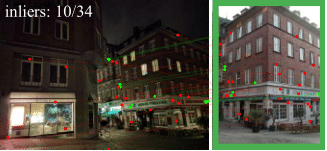}
\end{minipage}

\begin{minipage}{\iwidth}
    \centering
    \includegraphics[width=0.98\linewidth]{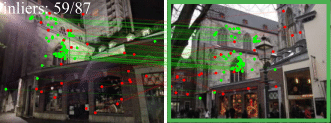}
\end{minipage}%
\begin{minipage}{\iwidth}
    \centering
    \includegraphics[width=0.98\linewidth]{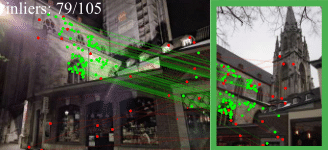}
\end{minipage}

\begin{minipage}{\iwidth}
    \centering
    \includegraphics[width=0.98\linewidth]{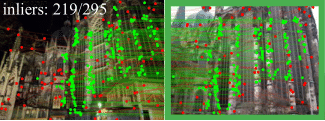}
\end{minipage}%
\begin{minipage}{\iwidth}
    \centering
    \includegraphics[width=0.98\linewidth]{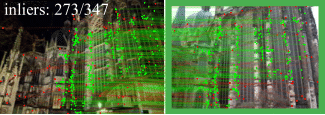}
\end{minipage}

\begin{minipage}{\iwidth}
    \centering
    \includegraphics[width=0.98\linewidth]{images/sift_aachen_compressed/SIFT_pca64_aachen_191533_compressed.pdf}
\end{minipage}%
\begin{minipage}{\iwidth}
    \centering
    \includegraphics[width=0.98\linewidth]{images/sift_aachen_compressed/SIFT_triplet64_aachen_191533_compressed.pdf}
\end{minipage}

\begin{minipage}{\iwidth}
    \centering
    \includegraphics[width=0.98\linewidth]{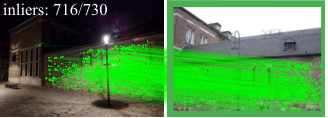}
\end{minipage}%
\begin{minipage}{\iwidth}
    \centering
    \includegraphics[width=0.98\linewidth]{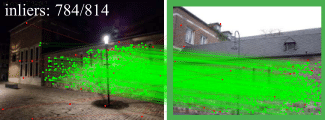}
\end{minipage}

\begin{minipage}{\iwidth}
    \centering
    \includegraphics[width=0.98\linewidth]{images/sift_aachen_compressed/SIFT_pca64_aachen_191555_compressed.pdf}
\end{minipage}%
\begin{minipage}{\iwidth}
    \centering
    \includegraphics[width=0.98\linewidth]{images/sift_aachen_compressed/SIFT_triplet64_aachen_191555_compressed.pdf}
\end{minipage}

\begin{minipage}{\iwidth}
    \centering
    \includegraphics[width=0.98\linewidth]{images/sift_aachen_compressed/SIFT_pca64_aachen_191752_compressed.pdf}
\end{minipage}%
\begin{minipage}{\iwidth}
    \centering
    \includegraphics[width=0.98\linewidth]{images/sift_aachen_compressed/SIFT_triplet64_aachen_191752_compressed.pdf}
\end{minipage}

\begin{minipage}{\iwidth}
    \centering
    \includegraphics[width=0.98\linewidth]{images/sift_aachen_compressed/SIFT_pca64_aachen_192213_compressed.pdf}
\end{minipage}%
\begin{minipage}{\iwidth}
    \centering
    \includegraphics[width=0.98\linewidth]{images/sift_aachen_compressed/SIFT_triplet64_aachen_192213_compressed.pdf}
\end{minipage}
\vspace{1mm}

\caption{\textbf{Localization with SIFT-PCA-64 and SIFT-Triplet-64 on Aachen Day-Night v1.1.} For each image pair, the left image is the query and the right image is the retrieved database image with the most inlier matches, as returned by PnP+RANSAC. SIFT-Triplet-64 can find more positive keypoint matches than SIFT-PCA-64 under different challenging circumstances. Best view in zoom and color.}
\label{fig:qual:Aachen}
%\vspace{-5mm}
\end{figure}
