# Supplementary material for: Learning-Based Dimensionality Reduction for Computing Compact and Effective Local Feature Descriptors
Source: arXiv:2209.13586 source file (2022-09-27)
Supplement: Supplementary file 2 [file sift_inloc.tex]

\begin{figure}[htb!]
\centering
\def\iwidth{.49\linewidth}

\begin{minipage}{\iwidth}
    \centering
    \small{SIFT-PCA-64}
\end{minipage}%
\begin{minipage}{\iwidth}
    \centering
    \small{SIFT-Triplet-64}
\end{minipage}

\begin{minipage}{\iwidth}
    \centering
    \includegraphics[width=0.98\linewidth]{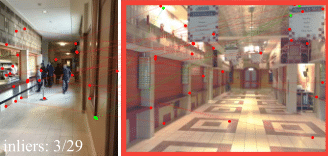}
\end{minipage}%
\begin{minipage}{\iwidth}
    \centering
    \includegraphics[width=0.98\linewidth]{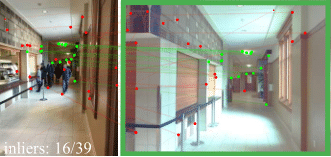}
\end{minipage}

\begin{minipage}{\iwidth}
    \centering
    \includegraphics[width=0.98\linewidth]{images/sift_inloc_compressed/SIFT_pca64_inloc_IMG_0949_compressed.pdf}
\end{minipage}%
\begin{minipage}{\iwidth}
    \centering
    \includegraphics[width=0.98\linewidth]{images/sift_inloc_compressed/SIFT_triplet64_inloc_IMG_0949_compressed.pdf}
\end{minipage}

\begin{minipage}{\iwidth}
    \centering
    \includegraphics[width=0.98\linewidth]{images/sift_inloc_compressed/SIFT_pca64_inloc_IMG_0971_compressed.pdf}
\end{minipage}%
\begin{minipage}{\iwidth}
    \centering
    \includegraphics[width=0.98\linewidth]{images/sift_inloc_compressed/SIFT_triplet64_inloc_IMG_0971_compressed.pdf}
\end{minipage}

\begin{minipage}{\iwidth}
    \centering
    \includegraphics[width=0.98\linewidth]{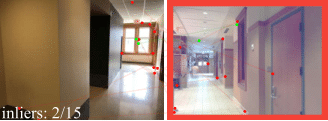}
\end{minipage}%
\begin{minipage}{\iwidth}
    \centering
    \includegraphics[width=0.98\linewidth]{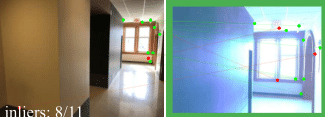}
\end{minipage}

\begin{minipage}{\iwidth}
    \centering
    \includegraphics[width=0.98\linewidth]{images/sift_inloc_compressed/SIFT_pca64_inloc_IMG_0833_compressed.pdf}
\end{minipage}%
\begin{minipage}{\iwidth}
    \centering
    \includegraphics[width=0.98\linewidth]{images/sift_inloc_compressed/SIFT_triplet64_inloc_IMG_0833_compressed.pdf}
\end{minipage}

\begin{minipage}{\iwidth}
    \centering
    \includegraphics[width=0.98\linewidth]{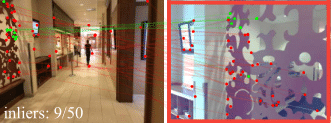}
\end{minipage}%
\begin{minipage}{\iwidth}
    \centering
    \includegraphics[width=0.98\linewidth]{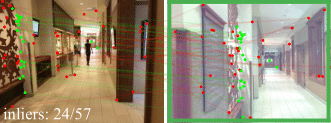}
\end{minipage}

\begin{minipage}{\iwidth}
    \centering
    \includegraphics[width=0.98\linewidth]{images/sift_inloc_compressed/SIFT_pca64_inloc_IMG_0863_compressed.pdf}
\end{minipage}%
\begin{minipage}{\iwidth}
    \centering
    \includegraphics[width=0.98\linewidth]{images/sift_inloc_compressed/SIFT_triplet64_inloc_IMG_0863_compressed.pdf}
\end{minipage}

\begin{minipage}{\iwidth}
    \centering
    \includegraphics[width=0.98\linewidth]{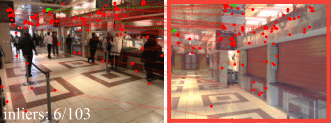}
\end{minipage}%
\begin{minipage}{\iwidth}
    \centering
    \includegraphics[width=0.98\linewidth]{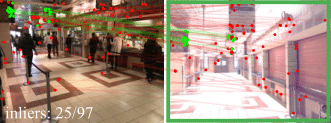}
\end{minipage}
\vspace{1mm}

\caption{\textbf{Localization with SIFT-PCA-64 and SIFT-Triplet-64 on InLoc.} Best view in zoom and color.}
\label{fig:qual:InLoc}
%\vspace{-5mm}
\end{figure}
